# Supplementary material for: Designing and Evaluating Presentation Strategies for Fact-Checked Content
Source: arXiv:2308.10220 source file (2023-12-24)
Supplement: Supplementary file 1 [file supp.tex]

% gender{[}T.gender\_male{]}                   & -7.9614  & 4.064 & -1.959 & 0.050 & -15.926 & 0.003  \\
% education\_adj{[}T.education\_2{]}           & 7.5143   & 6.677 & 1.125  & 0.260 & -5.572  & 20.600 \\
% education\_adj{[}T.education\_3\_4{]}        & -5.3665  & 7.005 & -0.766 & 0.444 & -19.096 & 8.363  \\
% websites{[}T.websites\_occasionally{]}       & -3.5781  & 5.662 & -0.632 & 0.527 & -14.675 & 7.519  \\
% websites{[}T.websites\_rarely{]}             & 7.0069   & 7.386 & 0.949  & 0.343 & -7.469  & 21.483 \\
% capability\_adj{[}T.capability\_2{]}         & 4.9572   & 5.448 & 0.910  & 0.363 & -5.721  & 15.636 \\
% capability\_adj{[}T.capability\_3{]}         & 5.0823   & 7.189 & 0.707  & 0.480 & -9.008  & 19.173 \\
% political\_adj{[}T.political\_independent{]} & -5.1052  & 6.863 & -0.744 & 0.457 & -18.557 & 8.346  \\
% political\_adj{[}T.political\_republican{]}  & 5.0222   & 4.927 & 1.019  & 0.308 & -4.634  & 14.678 \\
% debunked{[}T.debunked\_1{]}                  & 0.3632   & 4.834 & 0.075  & 0.940 & -9.110  & 9.837  \\
% debunked{[}T.debunked\_2{]}                  & -7.7353  & 6.074 & -1.274 & 0.203 & -19.640 & 4.169  \\
% debunked{[}T.debunked\_3{]}                  & -18.1271 & 8.674 & -2.090 & 0.037 & -35.127 & -1.127 \\
% debunked{[}T.debunked\_4{]}                  & -4.9829  & 6.571 & -0.758 & 0.448 & -17.862 & 7.897  \\
% age\_int                                     & 4.9810   & 2.251 & 2.213  & 0.027 & 0.569   & 9.393  \\
% bos                                          & 3.7031   & 1.736 & 2.133  & 0.033 & 0.301   & 7.105  \\
% cmq                                          & 1.2555   & 2.184 & 0.575  & 0.565 & -3.026  & 5.537  \\
